# Supplementary material for: Systematic Modification of Functionality in Disordered Elastic Networks Through Free Energy Surface Tailoring
Source: arXiv:2207.03861 source file (2022-08-15)
Supplement: Supplementary file 1 [file Network_CV_FEST_new_copy_to_PhysRevX_SI.pdf]

# Supporting Information for Systematic Modification of Functionality in Disordered Elastic Networks Through Free Energy Surface Tailoring

Dan Mendels,<sup>1</sup> Fabian Byléhn,<sup>1</sup> Timothy W. Sirk,<sup>2</sup> and Juan J. de Pablo<sup>1</sup>

<sup>1</sup>*Pritzker School of Molecular Engineering, University of Chicago,  
5640 S. Ellis Avenue, Chicago, Illinois USA 60637*

<sup>2</sup>*Polymers Branch, U.S. CDC Army Research Laboratory,  
Aberdeen Proving Ground, Maryland 21005, United States*

# Rotation of the 2d plane spanned by the top HLDA eigenvectors

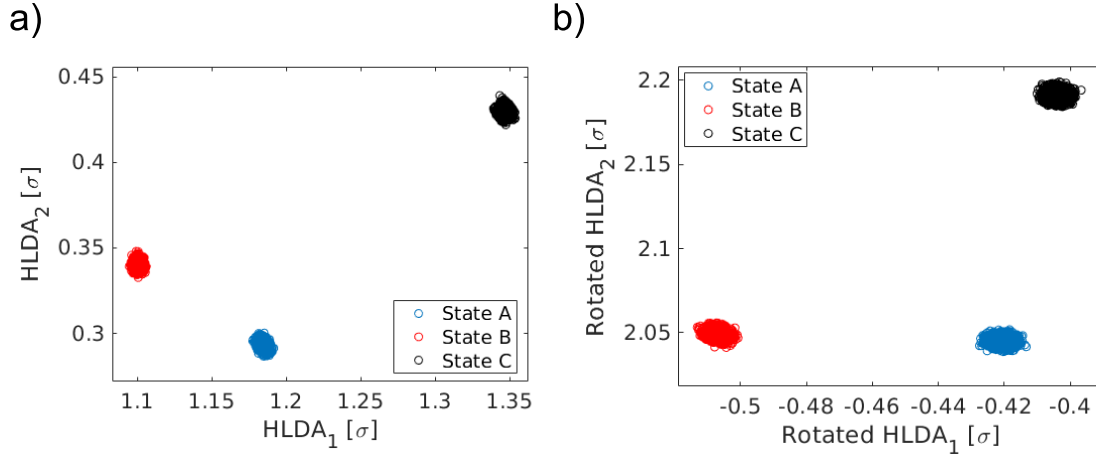

FIG. S1. a) Projection of the data sampled in the training simulations of the three considered states (A being the inactivated state, B the activated state, and C the inhibiting state) on the plane spanned by the top two HLDA eigenvectors. b) The HLDA eigenvector plane after rotation. It can be seen that states A and B are now predominantly separated with respect to the rotated  $HLDA_2$ , while states A and C are predominantly separated with respect to the rotated  $HLDA_1$ .

Example of time dependence behavior in a WTMD simulation in which  $d_s$  is the biased CV

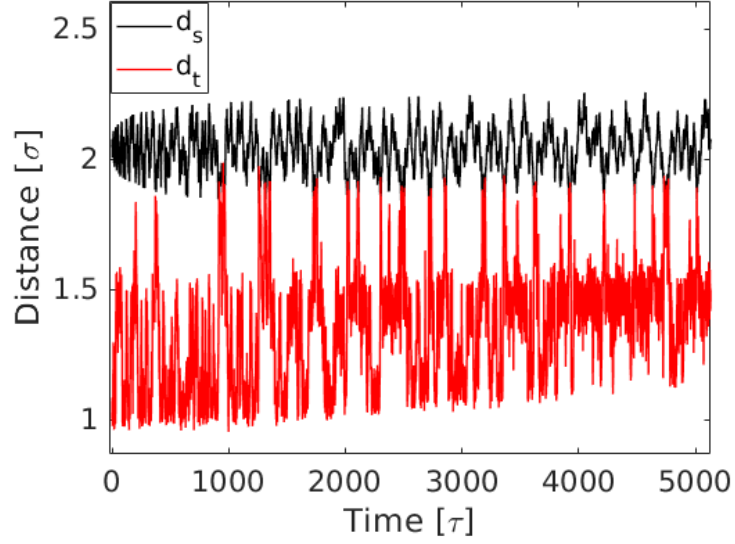

FIG. S2. Time dependence excerpt from a WTMD simulation run at  $T = 8.6 \cdot 10^{-6}$  ( $k_B = 1$ ) in which  $d_s$ , the distance between the source nodes is the biased CV. It can be seen that upon passing a threshold value, the allosteric response of the target beads (measured by the distance between them,  $d_t$ ) is triggered.

# **Time dependence behavior in WTMD simulations for a pristine and modified network**

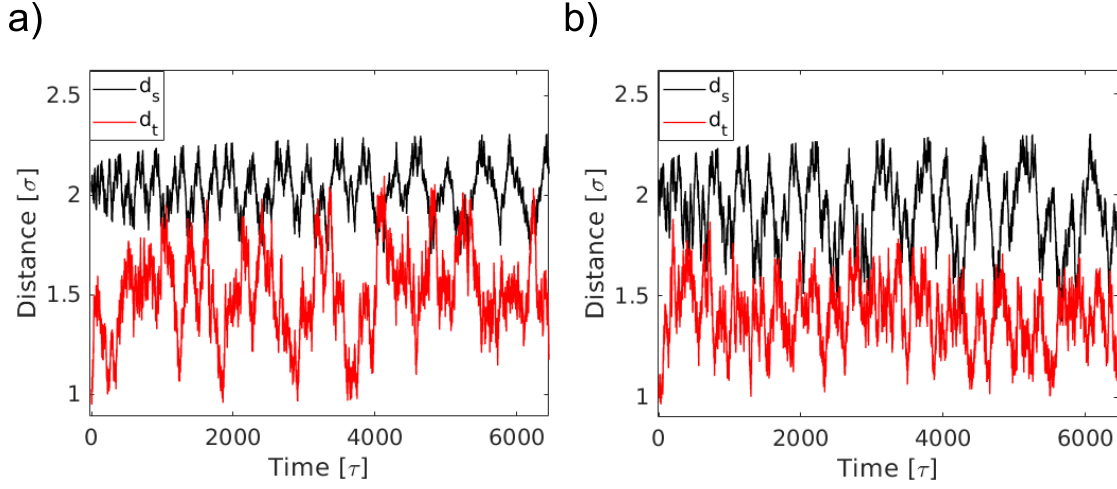

FIG. S3. a) Time dependence excerpt from a WTMD simulation of the pristine network run at  $T = 4.3 \cdot 10^{-5}$  in which  $d_s$ , the distance between the source nodes is the biased CV. It can be seen that upon passing a threshold value, the allosteric response of the target beads (measured by the distance between them,  $d_t$ ) is triggered. b) Time dependence excerpt from a WTMD simulation run at  $T = 4.3 \cdot 10^{-5}$  of a modified network for which the bonds ranked 12-27 in the HLDA<sub>1</sub> weight hierarchy were weakened. As can be seen the activated state is inhibited in the modified network whereby for values  $d_s < 1.7$  the target beads do not access the activated region of  $d_t > 1.7$

Equation for the calculation of the free energy difference  $\Delta F$  between any two states A and B

$$\Delta F = -\frac{1}{\beta} \log \frac{\int_A d\mathbf{s} e^{-\beta F(\mathbf{s})}}{\int_B d\mathbf{s} e^{-\beta F(\mathbf{s})}} \quad (\text{S1})$$
